# Supplementary material for: A practical example for the non-linear Bayesian filtering of model parameters
Source: arXiv:1807.08713 source file (2019-02-22)
Supplement: Supplementary file 1 [file appendix.tex]

\section*{Appendix A: Quantities of interest and weak representations of measures} \label{Subs_Integrals}
When considering measures $(\mu_t)_{t=1}^\infty$, we are typically interested in computing the expected value of a measurable and $\mu_t$-integrable ($t \geq 1$) \emph{quantity of interest} $f : X \rightarrow \mathbb{R}$ with respect to the probability measures $(\mu_t)_{t=1}^\infty$, that is $$\mu_t(f) := \int f \mathrm{d}\mu_t, \ \ t \geq 1.$$
Consider for instance the following examples of quantities of interest.
\begin{example} \label{EXAm_QoI}
Let $t \geq 1$.
\begin{enumerate}
\item Let $f(x) := x_i$ be the canonical projection on the $i$'s coordinate of $x$. Then, $\mu_t(f)$ is the \emph{mean} of the $i$'s marginal density of $\mu_t$. Moreover, $\mu_t(f^k)$ for $k \in \mathbb{N}$ is the $k$-th moment of the same marginal.
\item Let $A \subseteq X$ be an event and let $f$ be given by
$$
f(x) = \begin{cases} 1, &\text{if } x \in A,\\
0, &\text{otherwise.}
\end{cases}
$$
Then, $\mu_t(f) =: \mu_t(A)$ is the \emph{probability of $A$}.
\end{enumerate}
\end{example}

The quantities of interest given in Example \ref{EXAm_QoI} are of independent interest. 
However, it is possible to use integrals with respect to functions like quantities of interest to fully represent a measure. 
\begin{proposition}
Let $\mu, \nu$ be two measures on $X$. Then $\mu = \nu$, if one of the following conditions holds:
\begin{enumerate}
\item $\mu(A) = \nu(A), A \subseteq X$ measurable,
\item $\mu(f) = \nu(f),$ for all bounded, measurable functions $f: X\rightarrow \mathbb{R}$,
\item $\mu(f) = \nu(f),$ for all bounded, continuous functions $f: X\rightarrow \mathbb{R}$,
\item $\mu(f) = \nu(f),$ for all bounded, Lipschitz-continuous functions $f: X\rightarrow \mathbb{R}$.
\end{enumerate}
\end{proposition}
Moreover, we can use these criteria to specify the convergence of a sequence of measures.
\begin{proposition} \label{Prop_Convergence}
Let $(\mu^M)_{M=1}^\infty$ be a sequence of measures and $\nu$ be a further measure on $X$. Then $\mu^M \rightarrow \nu$, as $M \rightarrow \infty$, 

\begin{enumerate}
\item in total variation, if one of the following conditions holds 
\begin{enumerate}
\item $\mu^M(A) \rightarrow \nu(A)$, as $M \rightarrow \infty$, for all $A \subseteq X$ measurable,
\item $\mu^M(f) \rightarrow \nu(f)$, as $M \rightarrow \infty$, for all bounded, measurable functions $f: X\rightarrow \mathbb{R}$,
\end{enumerate}
\item  weakly, if it convergence in total variation or if one of the following conditions holds 
\begin{enumerate}
\item $\mu^M(f) \rightarrow \nu(f)$, as $M \rightarrow \infty$, for all bounded, continuous functions $f: X\rightarrow \mathbb{R}$,
\item $\mu^M(f) \rightarrow \nu(f)$, as $M \rightarrow \infty$, for all bounded, Lipschitz-continuous functions $f: X\rightarrow \mathbb{R}$.
\end{enumerate}
\end{enumerate}
\end{proposition}

Thus, instead of discussing measures, we can focus on integrals of functions with respect to these measures.

\section*{Appendix B: Source code of the ParticleApproximation class}

\lstinputlisting[caption={Python file {\fontfamily{txtt}\selectfont particle\_approximation.py}.},captionpos=b]{figures/particle_approximation.py}

%%% Local Variables:
%%% mode: latex
%%% TeX-master: "../main"
%%% End:
